# Supplementary material for: Periodic steady state and interference in a periodically driven quantum system
Source: arXiv:1204.5084 ancillary file (2012-11-16)
Supplement: Supplementary file 1 [file SM2.pdf]

# Periodic steady state and interference in a periodically driven quantum system - Supplementary material

Angelo Russomanno[1,2], Alessandro Silva[3], Giuseppe E. Santoro[1,2,3]
[1] *SISSA, Via Bonomea 265, I-34136 Trieste, Italy*
[2] *CNR-IOM Democritos National Simulation Center, Via Bonomea 265, I-34136 Trieste, Italy*
[3] *International Centre for Theoretical Physics (ICTP), P.O.Box 586, I-34014 Trieste, Italy*

PACS numbers: 75.10.Pq, 05.30.Rt, 03.65.-w

## I. BOGOLIUBOV-DE GENNES EQUATIONS FOR THE INHOMOGENOUS CASE IN A NUTSHELL

In this section we wolud like to give some flavour of what happens in the inhomogenous case, referring for more details to the discussion of Ref.[1]. In this case we can write the Hamiltonian of Eq. (2) in the main text in the form

$$\hat{H}(t) = \sum_{ij=1}^{2L} \hat{\Psi}_i^\dagger \widetilde{H}_{ij}(t) \hat{\Psi}_j \,. \tag{1}$$

$\widetilde{H}_{ij}$ is a $2L \times 2L$ Hermitean matrix containing the parameters of Eq. (2) in the main text, $\Psi_j$ are the $2L$ components of a Nambu spinor defined as $\Psi_j = c_j$ and $\Psi_{L+j} = c_j^\dagger$ for $1 \leq j \leq L$, where $c_j$ are the $L$ fermionic operators stemming from the Jordan-Wigner transformation. Let us focus for now on time 0. Following Bogoliubov, we can apply an unitary transformation

$$\hat{\mathbf{\Psi}} = \begin{pmatrix} u_d(0) & v_d^*(0) \\ v_d(0) & u_d^*(0) \end{pmatrix} \hat{\mathbf{\Phi}}_d(0) \tag{2}$$

($u_d(0)$ and $v_d(0)$ are $L \times L$ matrices) to the Hamiltonian of Eq. (1) and diagonalize it recasting it in the form

$$\hat{H}(0) = \sum_{\alpha=1}^{L} E_\alpha(0) \left( \gamma_{d\,\alpha}(0)^\dagger \gamma_{d\,\alpha}(0) - \gamma_{d\,\alpha}(0) \gamma_{d\,\alpha}(0)^\dagger \right) \,, \tag{3}$$

where the $\gamma_{d\,\alpha}(0)$ are quasiparticle Fermionic operators and the spinor $\hat{\Phi}(0)$ is defined in terms of them as $\Phi_{d\,\alpha}(0) = \gamma_{d\,\alpha}(0)$ and $\Phi_{d\,L+\alpha}(0) = \gamma_{d\,\alpha}(0)^\dagger$ for $1 \leq \alpha \leq L$. Therefore, also in the inhomogenous case the system can be described in terms of Fermionic quasi-particles, we will see soon that this will be true not only in the static but also in the dynamic case. We assume to start in the ground state $|\mathrm{GS}(0)\rangle$. It is the state with least energy $E_{\mathrm{GS}}(0) = -\sum_\alpha E_\alpha(0)$ and in it, for all values of $\alpha$, $\langle \mathrm{GS}(0)| \gamma_{d\,\alpha}(0)^\dagger \gamma_{d\,\alpha}(0) |\mathrm{GS}(0)\rangle = 0$ and, consistently with the Fermionic commutation rules $\langle \mathrm{GS}(0)| \gamma_{d\,\alpha}(0) \gamma_{d\,\alpha}(0)^\dagger |\mathrm{GS}(0)\rangle = 1$[12]. To discuss the dynamics of this system, through an unitary time dependent transformation

$$\hat{\mathbf{\Psi}} = \begin{pmatrix} u(t) & v^*(t) \\ v(t) & u^*(t) \end{pmatrix} \hat{\mathbf{\Phi}}(t) \,, \tag{4}$$

we introduce $L$ fermionic time-dependent quasiparticle operators $\gamma_\alpha(t)$ ($\Phi_\alpha(t) = \gamma_\alpha(t)$ and $\Phi_{L+\alpha}(t) = \gamma_\alpha(t)^\dagger$ for $1 \leq \alpha \leq L$) making the Bogoliubov time-dependent *Ansatz* which amounts to assume that the averages of all possible quadratic operators like $\langle \gamma_\alpha(t) \gamma_\beta(t) \rangle_t$ are constant and equal to $\langle \gamma_{d\,\alpha}(0) \gamma_{d\,\beta}(0) \rangle_0$. This *Ansatz* can be implemented by assuming that the operators $\gamma_\alpha(t)$ in the *Heisenberg representation* are constant and equal to $\gamma_{d\,\alpha}(0)$

$$\gamma_{\alpha\,H}(t) = \gamma_{d\,\alpha}(0) \,. \tag{5}$$

With this assumption, we have the evolution equations

$$i\hbar \partial_t \gamma_\alpha(t) = -\left[ \gamma_\alpha(t), H(t) \right] \,. \tag{6}$$

From this equality, we can find the evolution equations for the coefficients $u_{i\,\alpha}$ and $v_{i\,\alpha}$ of :the transformation in Eq. (4). If we apply to Eq. (6) the inverse of this transformation, substitute the explicit form Eq. (1) of the Hamiltonian and use the Fermionic commutation rules among the operators $c_j$, we obtain the Bogoliubov-De Gennes evolution equations

$$i \frac{d}{dt} \begin{pmatrix} u\,(t) \\ v\,(t) \end{pmatrix} = 2\widetilde{H}\,(t) \begin{pmatrix} u\,(t) \\ v\,(t) \end{pmatrix} \,. \tag{7}$$

The initial conditions are given by $u(0) = u_d(0)$ and $v(0) = v_d(0)$, where $v_d(0)$ and $u_d(0)$ have been defined in Eq. (2) and the matrix $\widetilde{H}(t)$ has been defined in Eq. (1). We can see that these equations are in a perfectly Schroedinger form, therefore we can apply to them the Floquet analysis we will discuss in the next section. It will allow us to find the periodic part of the observbales, thanks to the Floquet modes, and to understand if the fluctuations around it will vanish asymptoptically, thanks to the Floquet spectrum which in this case has to be mostly continuous.

To conclude this section, we show an example of how to write the average value of an observable in terms of the coefficients $u_{i\,\alpha}$ and $v_{i\,\alpha}$ whose evolution is described in Eq. (7). We take for instance the transverse magnetization

$$\hat{m} = \frac{1}{L} \sum_{j=1}^{L} \sigma_j^x = \frac{1}{L} \sum_{j=1}^{L} \left( 1 - 2c_j^\dagger c_j \right) \tag{8}$$

where the second equality comes from the Jordan-Wigner transformation. Evaluating the average value at time $t$

and applying the inverse of Eq. (4) we find, exploiting the constancy of the operator

$$m(t) = 1 - \frac{1}{L}\sum_{j,\,\alpha=1}^{L}\big(|u_{j\,\alpha}(t)|^2 \left\langle \gamma_{d\,\alpha}(0)^\dagger \gamma_{d\,\alpha}(0)\right\rangle_0 + |v_{j\,\alpha}(t)|^2 \left\langle \gamma_{d\,\alpha}(0)\gamma_{d\,\alpha}(0)^\dagger\right\rangle_0\big)\,. \quad (9)$$

In the case we discuss, in which we start from the ground state wher $\left\langle \gamma_{d\,\alpha}(0)^\dagger \gamma_{d\,\alpha}(0)\right\rangle_0 = 0$ and $\left\langle \gamma_{d\,\alpha}(0)\gamma_{d\,\alpha}(0)^\dagger\right\rangle_0 = 0$, but there are other possibilities, like a thermal density matrix. Moreover, by expanding the $u_{j\,\alpha}(t)$, $v_{j\,\alpha}(t)$ in Floquet modes, we can easily isolate the periodic part.

## II. FLOQUET THEORY AND TIME EVOLUTION OPERATOR IN THE HOMOGENOUS CASE

In this section we review Floquet theory and, to keep the presentation simple, we show explicitly how to apply it to the homogenous factorizable case. The discussion of the inhomogenous case is very similar in spirit but calculations are more lengthy because we have to deal with the $2L \times 2L$ system of linear differential equations Eq. (7), to which the Floquet analysis applies unaltered.

Floquet theory[2–4] is the analogue for time periodic Hamiltonians of Bloch theory for space periodic ones. Its main statement is that there exists a basis of solutions of the Schrödinger equation which are periodic in time up to a phase (like Bloch waves are in space)

$$|\Psi_\alpha(t)\rangle = \mathrm{e}^{-i\mu_\alpha t}\,|\Phi_\alpha(t)\rangle\,. \quad (10)$$

The states $|\Psi_\alpha(t)\rangle$ are named Floquet states, the real quantities $\mu_\alpha$ Floquet exponents or quasienergies and the states $|\Phi_\alpha(t)\rangle = |\Phi_\alpha(t+\tau)\rangle$ Floquet modes. This theory allows us to write the time evolution operator for a generic time periodic problem in the form

$$\hat{U}(t,0) = \sum_\alpha \mathrm{e}^{-i\mu_\alpha t}\,|\Phi_\alpha(t)\rangle\,\langle\Phi_\alpha(0)|\,. \quad (11)$$

Thanks to this formula and the periodicity of the Floquet modes, for $t = n\tau + \delta t$ with $n \in \mathbf{N}$ and $0 < \delta t < \tau$, we can write the time evolution operator as[4]

$$\hat{U}(t,0) = \hat{U}(\delta t, 0)\hat{U}^n(\tau,0)\,. \quad (12)$$

This simplifies numerical calculations. Notice also that $\hat{U}(\tau,0) = \sum_\alpha \mathrm{e}^{-i\mu_\alpha\tau}\,|\Phi_\alpha(0)\rangle\,\langle\Phi_\alpha(0)|$, implying that $|\Phi_\alpha(0)\rangle$ are eigenvectors of $\hat{U}(\tau,0)$ with eigenvalues $\mathrm{e}^{-i\mu_\alpha\tau}$.

Let us now discuss the practical implementation of these results for our problem in the homogeneous case. We can restrict ourselves to study the time evolution in each two dimensional subspace $k$. The Hamiltonian of this problem in the basis $\{c_k^\dagger c_{-k}^\dagger\,|0\rangle\,, |0\rangle\}$ is given by

$$H_k(t) = \begin{pmatrix} \cos k - h(t) & -i\sin k \\ i\sin k & -\cos k + h(t)\end{pmatrix}\,. \quad (13)$$

To obtain the time evolution operator we evolve numerically (using 4th order Runge-Kutta) with this Hamiltonian the state $\begin{pmatrix}1, & 0\end{pmatrix}^t$ (representing the state $c_k^\dagger c_{-k}^\dagger\,|0\rangle$ in the chosen basis) till time $\tau$ sampling the evolution with an appropriate mesh. Let $\begin{pmatrix} u_k^{(1)}(t), & v_k^{(1)}(t)\end{pmatrix}^t$ be the evolved vector at time $t$ . We can easily verify that if $\begin{pmatrix} u_k^{(1)}(t), & v_k^{(1)}(t)\end{pmatrix}^t$ solves the Bogoliubov-De Gennes system of differential equations $i\hbar\begin{pmatrix}\dot{u}_k \\ \dot{v}_k\end{pmatrix} = H_k(t)\begin{pmatrix}u_k \\ v_k\end{pmatrix}$ with initial condition $\begin{pmatrix}1, & 0\end{pmatrix}^t$, also $\begin{pmatrix} -v_k^{(1)*}(t), & u_k^{(1)*}(t)\end{pmatrix}^t$ is a solution but with initial condition $\begin{pmatrix}0, & 1\end{pmatrix}^t$. Therefore we can write in the chosen basis

$$U_k(t,0) = \begin{pmatrix} u_k^{(1)}(t) & -v_k^{(1)*}(t) \\ v_k^{(1)}(t) & u_k^{(1)*}(t)\end{pmatrix}\,. \quad (14)$$

In the inhomogenous case, we aim to find the evolution matrix $U(t,0)$ of the $2L \times 2L$ Bogoliubov de Gennes equations Eq. (7) and, with an argument very similar to the one just presented, we can restrict to solve those equations for only $L$ different initial conditions $\big(\underbrace{1,\ldots,0}_L\big|\underbrace{0,\ldots,0}_L\big)^t, \ldots, \big(\underbrace{0,\ldots,1}_L\big|\underbrace{0,\ldots,0}_L\big)^t$. When we diagonalize the evolution matrix $U(\tau,0)$ in the general case, which can be written as $\oplus_{k>0}U_k(\tau,0)$ in the homogenous case, we obtain the quasienergies as phases of the eigenvalues. For numerical reasons, it is better to diagonalize the Hermitian matrix

$$A = -i\,(\mathbf{1} - U(\tau,0))\,(\mathbf{1} + U(\tau,0))^{-1}\ ; \quad (15)$$

the Floquet quasienergies are obtained from the $2L$ eigenvalues $a_\alpha$ of this matrix as $\mu_\alpha = \frac{\omega_0}{\pi}\,\mathrm{atan}\,a_\alpha$. In the homogenous case, the Floquet quasienergies are labeled by the allowed values of $k$ and can be written explicitly, in terms of the parameters of Eq. (14)

$$\mu_k^\pm = \pm\frac{\omega_0}{\pi}\,\mathrm{atan}\sqrt{\frac{1-\Re\,u_k^{(1)}(\tau)}{1+\Re\,u_k^{(1)}(\tau)}}\,. \quad (16)$$

The Floquet modes at time 0 are the eigenvectors of $U(\tau,0)$ and in the homogenous case can be written explicitly as the eigenvectors of Eq. (14)

$$\left|\phi_k^{\pm}(t=0)\right\rangle = \frac{1}{\sqrt{2\left(1-\left(\Re u_k^{(1)}(\tau)\right)^2\right) \mp 2\Im u_k^{(1)}(\tau)\sqrt{1-\left(\Re u_k^{(1)}(\tau)\right)^2}}} \begin{pmatrix} i v_k^{(1)}(\tau)^* \\ -\Im u_k^{(1)}(\tau) \pm \sqrt{1-\left(\Re u_k^{(1)}(\tau)\right)^2} \end{pmatrix} . \quad (17)$$

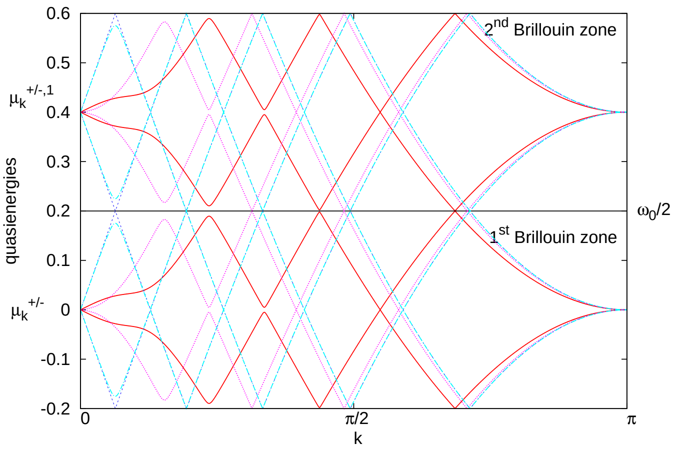


FIG. 1: Quasienergies vs $k$ for $\omega_0 = 0.4$ and $A = 0$ (blue short-dashed line), $A = 0.05$ (light-blue long-dashed line), $A = 0.5$ (purple dotted line), $A = 1$ (red solid line) in the first two Brillouin zones. We notice that when $A$ is small the degeneracies of the $A = 0$-cas are shifted a bit and a small gap opens. When $A$ is increased further, the quasi-degeneracies at small $k$ disappear while the ones at large $k$ are shifted but with relatively small gaps.

The Floquet modes at subsequent times are obtained through the formula

$$\left|\phi_k^{\pm}(t)\right\rangle = e^{i\mu_k^{\pm} t}\hat{U}_k(t,0)\left|\phi_k^{\pm}(0)\right\rangle . \quad (18)$$

We notice that the Floquet modes are defined up to a periodic phase. If we replace $\left|\phi_k^{\pm}(t)\right\rangle$ with $\left|\phi_k^{\pm,l}(t)\right\rangle = e^{il\omega_0 t}\left|\phi_k^{\pm}(t)\right\rangle$ (with $l \in \mathbf{N}$) we obtain an equally valid set of Floquet modes. Under this operation the quasienergies will be shifted

$$\mu_k^{\pm} \to \mu_k^{\pm,l} = \mu_k^{\pm} + l\,\omega_0 . \quad (19)$$

Therefore, like the electron quasimomenta in periodic potentials, quasienergies are defined up to translations of an integer number of $\omega_0$. We can define a first Brillouin zone $[-\omega_0/2,\, \omega_0/2]$ and restrict our quasienergies in it. Two quasienergies are degenerate if they coincide up to translations of an integer number of $\omega_0$. In Fig. 1 we see some examples of quasienergies vs. $k$ in the Homogenous case in the first two Brillouin zones. The short-dashed blue line shows the Floquet exponents with $A \to 0$ (vanishing driving amplitude). In this limit the quasienergies (up to translations of $\omega_0$) are the eigenvalues of the critical $\hat{H}_k$

$$\mu_{k,0}^{\pm,l} = \pm 2\sin\left(\frac{k}{2}\right) + l\,\omega_0 . \quad (20)$$

The degeneracy condition is therefore

$$4\sin\left(\frac{k}{2}\right) = n\omega_0 \quad (21)$$

for some integer $n$. We notice that this is an $n$-photon resonance condition. If we increase a bit the driving amplitude $A$, a gap opens and the resulting quasi-degeneracies are shifted. By further increasing the driving amplitude $A$, the quasi-degeneracies at small $k$ disappear, while the ones at large $k$ undergo a smaller influence: they are shifted but the gaps are kept narrow. These narrow gaps will be important when we will discuss the contribution of the modes with large $k$ to the quantities shown in Fig. 2 in the main text and Fig. 2 here. To see why the quasienergies behave so differently at small and large $k$ when $A$ increases, it is useful to observe that they are obtained (as shown in Eq. (16)) by diagonalizing the operator $U_k(\tau,0)$ which, in terms of the Hamiltonian Eq. (13), can be written as

$$U_k(\tau,0) = \overleftarrow{\mathrm{T}}\exp\left(-i\int_0^\tau \mathrm{d}t\, H_k(t)\right) . \quad (22)$$

If we apply the change of reference frame

$$|\psi_k(t)\rangle = V(t)\left|\widetilde{\psi}_k(t)\right\rangle \quad \text{with} \quad V(t) = e^{-iA\sin(\omega_0 t)\sigma^z/\omega_0} \quad (23)$$

we can see that the mode $k$ time evolution operator can be written as

$$U_k(\tau,0) = \overleftarrow{\mathrm{T}}\exp\left(-i\int_0^\tau \mathrm{d}t\, \widetilde{H}_k(t)\right) . \quad (24)$$

where the Hamiltonian in the new reference frame is defined as

$$\widetilde{H}_k(t) \equiv \sigma^z(1-\cos k) + \sin k\,\sigma^y \exp\left(2iA\frac{\sin(\omega_0 t)}{\omega_0}\sigma^z\right) . \quad (25)$$

The modes for which the driving amplitude $A$ has a small influence on the corresponding quasienergies, therefore, are the ones for which the second term of this Hamiltonian can be neglected. These modes obey the condition

$\pi/2 \ll k < \pi$: they are the large-$k$ modes, as we have noticed before.

In Fig. 9 we report the Floquet quasienergies in the first Brillouin zone for an example of inhomogenous case. Also here we can see that the Floquet spectrum is symmetric around zero thanks to the vanishing trace of the matrix $\widetilde{H}(t)$ in the Bogoliubov-de Gennes equations Eq. (7).

## III. DECAYING TRANSIENT AND PERIODIC BEHAVIOUR

In this section we discuss in more detail the convergence to the periodic steady state for the homogeneous spin chain model considered in the main text. We characterize the operators which become periodic and show that the spin correlators are among them and, in order to exemplify, we will discuss in some detail the case of the transverse magnetization.

The observables which reach the periodic steady state are those described by an operator $\hat{b}(t)$ (constant in time or time-periodic) whose average can be expressed as $b(t) = \langle\Psi(t)|\,\hat{b}(t)\,|\Psi(t)\rangle = (1/L)\sum_{k>0}^{\rm ABC}\langle\Psi(t)|\,\hat{B}_k(t)\,|\Psi(t)\rangle$, where $\hat{B}_k(t)$ has matrix elements only within the 2-dim space $\{c_k^\dagger c_{-k}^\dagger\,|0\rangle\,,|0\rangle\}$. To this kind of operator we can apply exactly the same argument based on the Riemann-Lebesgue lemma which we use in the main thext to show that $e\,(t)$ synchronizes. As done for this observable, we can see that there is a diagonal periodic part $b^{\rm per}\,(t)$ and an out of diagonal part $b^{\rm tr}(t)$ which vanishes after a transient. This vanishing can be seen very well in the high frequency limit $\omega_0 \to \infty$. In this limit, diagonalizing the Shirley-Floquet Hamiltonian[2–4], we can see that, for each $k$, the Floquet modes are the critical ($h = h_c = 1$) eigenstates of the $k$ component of the Hamiltonian, and the quasienergies are the corresponding eigenvalues $\pm 2\sin{(k/2)}$. Physically this means that in this limit the oscillations are so fast that the system does not feel the driving. In this limit we can write analytical formulas for $b^{\rm per}(t)$ and $b^{\rm tr}(t)$, and notice that $b^{\rm tr}(t)$ goes to zero as $t^{-1/2}$ when $\hat{b}(t) = \hat{m}$ or $\hat{b}(t) = \hat{e}(t)$. For lower frequencies we have found numerically that for both these observables the transient term $b^{\rm tr}(t)$ goes to zero either as $t^{-1/2}$ when $\omega_0 > 4J$ or as $t^{-3/2}$. The behaviour for large frequency is confirmed by the results for the transverse magnetization analyzed in Ref.[5].

We notice that the argument leading to the periodicity of $b\,(t)$ can be applied also to the spin correlators. Thanks to the Jordan-Wigner transformation[6] and to Wick's theorem, these correlators can be expressed as sums of products of the quantities[7]

$$\begin{aligned} G_{jl}(t) &= \langle\Psi(t)|\,c_j^\dagger c_l\,|\Psi(t)\rangle \\ F_{jl}(t) &= \langle\Psi(t)|\,c_j c_l\,|\Psi(t)\rangle\,. \end{aligned} \quad (26)$$

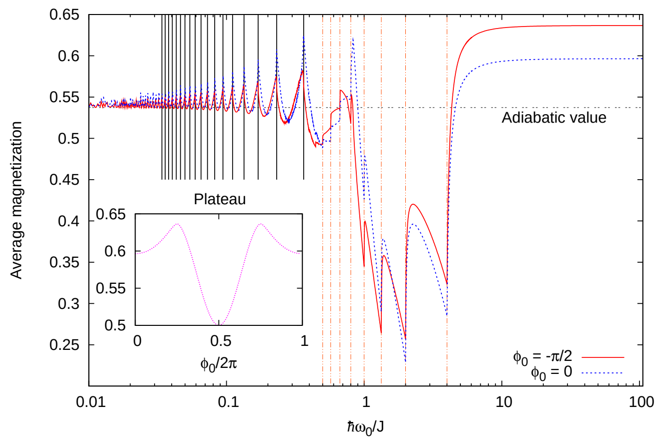


FIG. 2: Average transverse magnetization $\overline{m}$ vs $\omega_0$ for two values of the initial phase $\varphi_0 = 0$ (blue dashed line), and $\varphi_0 = -\pi/2$ (red solid line). (Inset) The magnetization-plateau $\overline{m}(\omega_0 \to \infty)$ vs $\varphi_0$.

where $c_j$ are the site-$j$ fermionic operators introduced by the Jordan-Wigner transformation. The first quantity, for example, in the thermodynamic limit can be written as

$$G_{jl} = \int_0^\pi \frac{{\rm d}k}{2\pi}\,\langle\psi_k(t)|\,c_k^\dagger c_k\,|\psi_k(t)\rangle\,{\rm e}^{ik(l-j)}\,, \quad (27)$$

which, thanks to the Floquet decomposition and the Riemann-Lebesgue lemma, becomes periodic after a transient.

Let us now focus on the transverse magnetization (see Eq. (8)),

$$m(t) = \frac{1}{L}\,\langle\Psi(t)|\sum_{j=1}^{L}\sigma_j^x\,|\Psi(t)\rangle\,.$$

Once again, this observable becomes periodic after a transient, as one should expect from its relation with the total energy $e(t)$, $\dot{e} = -\dot{h}\,m/2$. The periodic part obviously dominates if we take infinite-time averages:

$$\overline{m} \equiv \lim_{\mathcal{T}\to\infty}\frac{1}{\mathcal{T}}\int_0^{\mathcal{T}}{\rm d}t\;m(t) = \frac{1}{\tau}\int_0^{\tau}{\rm d}t\;m^{\rm per}(t)\,.$$

Fig. 2 shows $\overline{m}$ versus $\omega_0$. In it we can see the memory of the initial state discussed in connection with Eq. (1) in the main text. It is exemplified showing results for two possible phases $\varphi_0$ of the field $h(t) = 1+\cos{(\omega_0 t+\varphi_0)}$ (the initial state is the ground state computed with the initial field): $\varphi_0 = 0$, and $\varphi_0 = -\pi/2$, when $H(0) = H_c$ is the critical Hamiltonian. We notice once again peaks of decreasing amplitude occurring at low frequencies when $J_0(2J/\hbar\omega_0) = 0$, and dips at $\hbar\omega_0/J = 4/p$ which are

discussed in detail in Section IV. The former are the analogues of the dynamical freezing peaks observed in Ref. 8 for larger values of the driving amplitude $A$. As we will discuss better later, the ($\varphi_0$-dependent) plateau arising at $\omega_0 \to \infty$, is due to the inability of the system to follow the driving at high frequency, where the Floquet modes quickly approach the critical eigenstates as $\hbar\omega_0/J > 4$.

There are two last remarks. First, the syncronization of the observables comes from a purely coherent dynamics and keeps memory of the initial state through the overlap factors $r_k^{\pm}$; this should be contrasted to what happens in the case of decoherence by an external environment[3,9], where the decay of the transient is exponential and all information on the initial state is lost: for each $k$-mode, the density matrix itself becomes periodic and diagonal in the Floquet basis. Second, the quantum uncertainty of operators of the same form of $\hat{b}$ vanishes in the thermodynamic limit like $1/\sqrt{L}$ where $L$ is the length of the chain. So, in the thermodynamic limit, such observables are well defined.

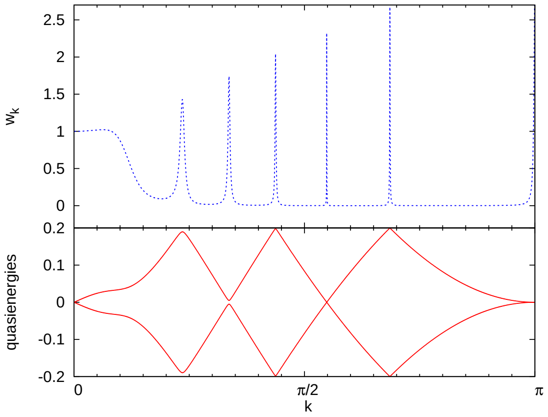


FIG. 3: (Upper panel) The integrand $w_k$ for $\omega_0 = 0.4$. Notice the peaks occurring at the values of $k$ for which the quasienergies are quasi-resonant (lower panel).

## IV. PEAKS AND DIPS

Setting now $A = 1$, let us justify the appearance of peaks and dips at the frequencies $4/p$ and at the zeros of $J_0(2/\omega_0)$ in all the considered quantities. We have to consider three quantities: the total work, the defect density after $\infty$ Landau-Zener crossings and the average of the magnetization. All these quantities can be written as an integral over $k$, in the thermodynamic limit. We analyze the behaviour of the integrand at different frequencies, especially the ones at which the peaks occur. The behaviour of this integrand depends, in all the considered cases, only on the overlaps $|r_k^\alpha|^2$ and on the Floquet modes $|\phi_k^\alpha(t)\rangle$.

For definiteness, let us consider first the total work and take $\varphi_0 = 0$. The last condition will give simpler analytical computations which can be generalized with some algebra to other values of $\varphi_0$. The total work is given by the difference of the energy at the end of the $n$-th cycle minus the corresponding ground state energy (which is the same as the initial energy) in the limit $n \to \infty$. In this limit the transient has died, so we have $w = e^{\rm per}(0) - e_{GS}(0)$ where we have used the periodicity of $e^{\rm per}(t)$. Using the formula for $e^{\rm per}(t)$ given in the main text we can express the work as an integral over $k$. Writing $\hat{e}(t) = \frac{1}{L}\sum_{k>0}^{\rm ABC} \hat{H}_k(t)$, we notice from Eq. (13) that $\hat{H}_k(t)$ has zero trace, so $\langle\phi_k^+(t)|\,\hat{H}_k(t)\,|\phi_k^+(t)\rangle = \langle\phi_k^-(t)|\,\hat{H}_k(t)\,|\phi_k^-(t)\rangle$ and we use that $|r_k^-|^2 + |r_k^+|^2 = 1$. In the end, defining $H_k^{++}(t) \equiv \langle\phi_k^+(t)|\,\hat{H}_k(t)\,|\phi_k^+(t)\rangle$ we can write

$$
\begin{aligned}
w &= \int_0^\pi \frac{{\rm d}k}{2\pi}\, w_k \quad \text{with} \\
w_k &= \left[\left(2\,|r_k^+|^2 - 1\right) H_k^{++}(0) + E_k(0)\right] \qquad (28)
\end{aligned}
$$

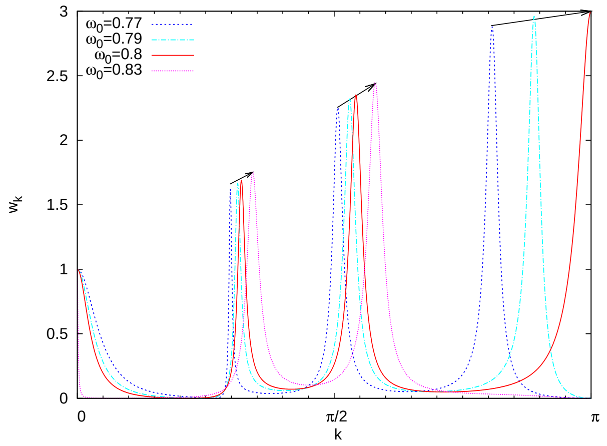


FIG. 4: The integrand $w_k$ for some frequencies around $\omega_0^{(5)} = 0.8$. The black arrows mark the direction of increasing frequency. Notice the uppermost right peak whose top is at $k = \pi$ for $\omega_0 = 0.8$ and then disappears.

Behind the features of Fig. 2a of the main text there is the behaviour of $w_k$ vs $k$ at different frequencies. When $\omega_0 < 4J$ there are quasi-resonances in the Floquet spectrum. Fixing $\omega_0$, $w_k$ shows some spikes at the values of $k$ for which the quasienergies are quasi-resonant (Fig. 3) as one empirically observes in the numerical results. As we have noticed before, for $\omega_0 > 4J$ there are no more quasi-degeneracies; correspondingly, the spikes in $w_k$ and peaks in $w$ disappear.

These spikes are important because it is just their be-

haviour which determines the peaks at frequency $\omega_0^{(p)} = 4/p$ in Fig. 2a of the main text. Choosing for instance $\omega_0^{(5)} = 0.8$, see Fig. 4, we can study what happens around this frequency. When $\omega_0$ grows, the spikes (and the corresponding Floquet quasi-degeneracies) move towards the right and, when $\omega_0 = \omega_0^{(5)}$, the top of a spike is just at $k = \pi$, the upper limit of the integral of Eq. (28). If we further increase the frequency, this spike goes beyond $k = \pi$ and does not contribute any more to the integral, which drops down abruptly.

The mechanism is the same for all $\omega_0^{(p)}$ and determines a peak at some frequency $\omega_0$ if at that frequency the top of a spike is at $k = \pi$. This is equivalent to saying that the mode at $k = \pi$ needs to have quasi-degenerate quasienergies. It turns out that at this point the quasi-degeneracy turns into a full degeneracy. Indeed, for $k = \pi$ we have:

$$H_{k=\pi}(t) = (2 - \cos(\omega_0 t))\, \sigma^z \tag{29}$$

where $\sigma$ are the Pauli matrices in the $k$ subspace with basis $\{|0\rangle, |k - k\rangle\}$. The time evolution operator over a period is $U_{k=\pi}(\tau, 0) = \mathrm{e}^{-2i\tau\sigma^z}$. Diagonalizing it we find that the quasienergies for the mode $k$ are

$$\mu_{k=\pi}^{\pm, l} = \pm 2 + l\, \omega_0 \ . \tag{30}$$

If we impose the resonance condition $\mu_k^{+,l} = \mu_k^{-,l'}$, we find $\omega_0 = 4/p$ with $p \in \mathbf{N}$.

Let us now study the dips at the frequencies for which $J_0(2/\omega_0)$ vanishes. We call these frequencies $\omega_0^{[q]}$ with $q \in \mathbf{N}$, corresponding to the $q$−th zero of $J_0$. The dip structure is seen very clearly for $\omega_0 \leq 0.5$ (the dips with $q \geq 2$) and we will focus on this frequency range. Here, the behaviour of $w$ depends very much on the modes with small $k$. We can see an example of that in Fig. 5.

We notice first that the modes with $k$ large give a modest contribution to $w_k$. For the considered frequencies and far from the quasi-resonances of the Floquet spectrum these modes are adiabatic and for them $w_k \equiv 0$. The quasi-resonances occurring in this $k$ range are very narrow, so $w_k \neq 0$ on very narrow spikes which contribute very modestly to the integral.

When $\omega_0$ is far from a dip, the low-$k$ modes give an important contribution: $w_k \to 1$ when $k \to 0$. The dips emerge at the frequencies $\omega_0^{[q]}$ because, in that case, the modes with small $k$ give a vanishing contribution to $w$. We can see this analytically by limiting our analysis to the values of $k$ for which the off-diagonal Hamiltonian term in Eq. (13) is such that $\Delta_k \ll \omega_0$. In this limit we can give an approximate analytical expression for $U_k(\tau, 0)$, which can be diagonalized to obtain $|\phi_k(0)\rangle$ and then $w_k$. We could use the Rotating Wave approximation[3,8,10], but we prefer to use first order perturbation theory which is somewhat simpler. Using that $\Delta_k = \sin k \approx k$, we approximate the Hamiltonian in

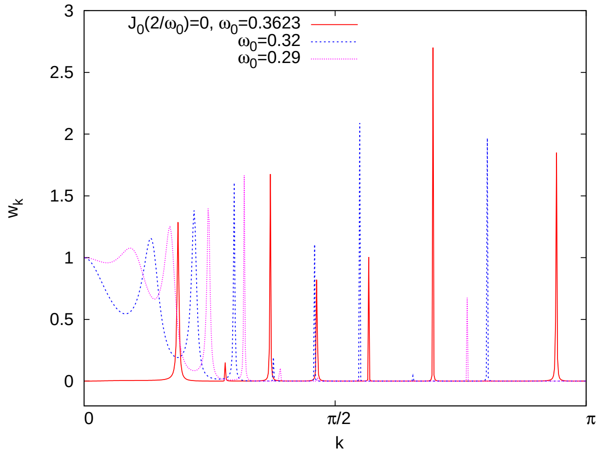


FIG. 5: The integrand $w_k$ vs $k$ for the dip frequency $\omega_0^{[2]} \simeq 0.3623$ and some frequency nearby. Notice that the first behaves very differently from the others for small $k$.

Eq. (13) to 2$^{\text{nd}}$ order in $k$

$$H_{k\ll 1}(t) \simeq \begin{pmatrix} \frac{k^2}{2} + \cos(\omega_0 t) & -ik \\ ik & -\frac{k^2}{2} - \cos(\omega_0 t) \end{pmatrix} . \tag{31}$$

Now we change reference frame, via the transformation

$$|\psi_k(t)\rangle = V(t) \left|\widetilde{\psi}_k(t)\right\rangle \quad \text{with} \quad V(t) = \mathrm{e}^{-i\sin(\omega_0 t)\sigma^z/\omega_0} . \tag{32}$$

In the new reference frame the evolution is given by the Schrödinger equation with the Hamiltonian

$$\widetilde{H}_{k\ll 1}(t) \simeq \sigma^z \frac{k^2}{2} + k\sigma^y \exp\left(2i\frac{\sin(\omega_0 t)}{\omega_0}\sigma^z\right) . \tag{33}$$

To first order in perturbation theory (using as perturbation the Hamiltonian in Eq. (33)) we obtain that the evolution operator over a period is

$$\begin{aligned} \widetilde{U}_{k\ll 1}(\tau, 0) &\simeq \mathbf{1} - i\int_0^\tau \widetilde{H}_{k\ll 1}(t)\,\mathrm{d}t \\ &= \mathbf{1} - i \begin{pmatrix} \frac{k^2}{2} & -ikJ_0\left(\frac{2}{\omega_0}\right) \\ ikJ_0\left(\frac{2}{\omega_0}\right) & -\frac{k^2}{2} \end{pmatrix} \tau. \end{aligned} \tag{34}$$

The application of first order perturbation theory is justified because we have assumed $k \ll \omega_0$ i.e. $k\tau \ll 1$. The time evolution operator in the initial reference frame is given by

$$U_{k\ll 1}(\tau, 0) = V(\tau)\, \widetilde{U}_{k\ll 1}(\tau, 0)\, V(0)^\dagger = \widetilde{U}_{k\ll 1}(\tau, 0) \ . \tag{35}$$

To obtain the Floquet modes we have therefore to diagonalize the operator of Eq. (34). It is obvious that this is equivalent to diagonalizing the matrix

$$k\left(\frac{k}{2}\sigma^z + J_0\left(\frac{2}{\omega_0}\right)\sigma^y\right) . \tag{36}$$

We can see that, fixing $\omega_0$, there are two different regimes for $w_k$: $\left|J_0\left(\frac{2}{\omega_0}\right)\right| \ll k \ll \omega_0$ and $k \ll \left|J_0\left(\frac{2}{\omega_0}\right)\right|$. In the first regime the matrix of Eq. (36) is $\propto \sigma^z$, therefore the Floquet modes are $\left|\phi_k^+(0)\right\rangle \simeq \left(\,1,\ 0\,\right)^t$ and $\left|\phi_k^-(0)\right\rangle \simeq \left(\,0,\ 1\,\right)^t$. Approximating to 0th-order in $k$, we find that in this limit $w_k = 0 + \mathcal{O}\left(k^2\right)$. To obtain this relation we have used that, to $2^{\rm nd}$ order in $k$, $E_k(0) \simeq 1 + k^2$ and the ground state of the $k$ mode (it is the state at time 0 necessary to compute the overlaps $|r_k^\alpha|^2$) is $|\psi_k(0)\rangle \simeq \left(\,ik,\ 1-k^2/2\,\right)^t$. In the second regime, instead, the matrix of Eq. (36) is $\propto \sigma^y$, therefore the Floquet modes are $\left|\phi_k^\pm(0)\right\rangle \simeq \frac{1}{\sqrt{2}}\left(\,\pm i,\ 1\,\right)^t$. At zero order in $k$, using the same approximations as before for $E_k(0)$ and $|\psi_k(0)\rangle$, we find $w_k = 1 + \mathcal{O}\left(k^2\right)$. We notice that the window in which the second regime holds tends to shrink when $\omega_0$ approaches a zero $\omega_0^{[q]}$ of $J_0\left(\frac{2}{\omega_0}\right)$ (see Fig. 6). So the range in which $w_k \simeq 1$ gets smaller and smaller, and the integral $w$ goes down till a minimum is reached at $\omega_0 = \omega_0^{[q]}$ where, even at the lowest $k$, $w_k \simeq 0$. These considerations suggest us that, as a very crude approximation, for $\omega_0 \le 0.5$, we can write

$$w \simeq \left|J_0\left(\frac{2}{\omega_0}\right)\right| \tag{37}$$

which qualitatively fits the behaviour of $w$ (see Fig. 7) reproducing also the $\sqrt{\omega_0}$ behaviour at low frequencies (when $\omega_0 \ll 2$ we have $J_0\left(\frac{2}{\omega_0}\right) \simeq \sqrt{\frac{\omega_0}{\pi}}\cos\left(\frac{2}{\omega_0} - \frac{\pi}{4}\right)$).

Finally we explain the high frequency plateau in Fig. 2a of the main text. This is due to the fact that for $\omega_0 \gg 4$, the Floquet modes at each $k$ are the eigenstates of $\hat{H}_k$ critical ($h = h_c = 1$) and the quasienergies are the corresponding eigenvalues. Therefore the modes are independent of time and frequency. The analytical formula for $w_k$ in the high frequency limit is

$$w_k(\omega_0 \to \infty) = E_k\left(0\right)\cos^2\left(\frac{k}{2} + \mathrm{atan}\left(\frac{\sin k}{h(0) - \cos k}\right)\right) \tag{38}$$

The discussion we have done for the work applies also to the density of defects after $\infty$ crossings of the quantum critical point and to the average magnetization[8]. Both these quantities show a behaviour very similar to the work as we can see in Fig. 2b of the main text and Fig. 2; the only difference is that they show peaks[8] and not dips at $\omega_0^{[q]}$ and the magnetization shows dips at the frequencies $\omega_0^{(p)}$. As for the work, both can be written as integrals over $k$; for the density of defects the integrand is

$$\nu_{d\,k} = \left[\left(2\left|r_k^+\right|^2 - 1\right)H_k^{++}(\tau/2) + 1\right] \tag{39}$$

while for the average magnetization it is

$$\overline{m}_k = \frac{1}{\tau}\int_0^\tau \mathrm{d}t\left[\left(2\left|r_k^+\right|^2 - 1\right)M_k^{++}(t)\right] \tag{40}$$

where $M_k^{++} \equiv 2\left\langle\phi_k^+(t)\right|\left(c_{-k}c_{-k}^\dagger - c_k^\dagger c_k\right)\left|\phi_k^+(t)\right\rangle$. Both these integrands show a behaviour very similar to $w_k$. We just discuss what happens at the frequencies $\omega_0^{[q]}$ where

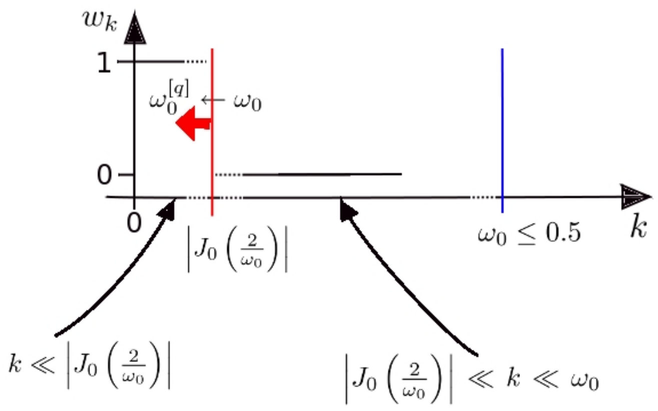


FIG. 6: The different behaviour of the integrand $w_k$ in the regimes $\left|J_0\left(\frac{2}{\omega_0}\right)\right| \ll k \ll \omega_0$ ($w_k \simeq 0$) and $k \ll \left|J_0\left(\frac{2}{\omega_0}\right)\right|$ ($w_k \simeq 1$). At the dip frequencies $\omega_0^{[q]}$, the window in which the second regime holds closes up and $w_k \equiv 0$ even for the smallest $k$'s.

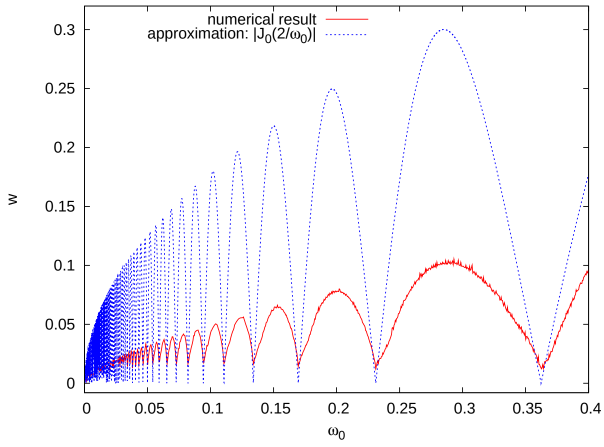


FIG. 7: The work $w$ for small frequency (red solid line) and the approximation $\left|J_0\left(\frac{2}{\omega_0}\right)\right|$ (blue dashed line) which fits at leas qualitatively.

we have peaks instead of dips. To explain these peaks is again crucial the behaviour of low-$k$ modes as we can see in Fig. 8. The considered range of frequencies is again $\omega_0 \leq 0.5$; in this range the high-$k$ modes behave adiabatically ($|\phi_k^{\pm}(t)\rangle$ are almost equal to instantaneous eigenstates of $\hat{H}_k(t)$) and, as $\omega_0$ changes, they give always the same contribution. (The high-$k$ modes do not behave adiabatically only near the Floquet quasi-resonances, where the integrands show narrow spikes which give a modest $\omega_0$ dependent contribution to the integrand.) The small-$k$ modes, instead, show a behaviour similar to that found for $w_k$. Now we have to find the Floquet modes at $\tau/2$ for $\nu_{d\,k}$ and at all times $0 < t \leq \tau$ for $\overline{m}_k$. To do that we have to diagonalize $U(t+\tau, t)$. Expanding $H_k(t)$ for small $k$ and applying first order perturbation theory as in Eq. (34), we find that the Floquet modes at time $t$ are eigenstates of the matrix

$$k \begin{pmatrix} \frac{k}{2} & -iJ_0\left(\frac{2}{\omega_0}\right)\mathrm{e}^{i\omega_0 t} \\ iJ_0\left(\frac{2}{\omega_0}\right)\mathrm{e}^{-i\omega_0 t} & -\frac{k}{2} \end{pmatrix} . \tag{41}$$

As before we have two regimes. The first is $\left|J_0\left(\frac{2}{\omega_0}\right)\right| \ll k \ll \omega_0$ where this matrix is approximately $\propto \sigma^z$ and the Floquet modes are $|\phi_k^+(t)\rangle \simeq \left(\begin{array}{cc} 1, & 0 \end{array}\right)^t$ and $|\phi_k^-(t)\rangle \simeq \left(\begin{array}{cc} 0, & 1 \end{array}\right)^t$. The second is $k \ll \left|J_0\left(\frac{2}{\omega_0}\right)\right|$ where the matrix is approximately $\propto \sigma^y \cos(\omega_0 t) + \sigma^x \sin(\omega_0 t)$ and $|\psi_k(t)\rangle \simeq \frac{1}{\sqrt{2}}\left(\begin{array}{cc} \pm i, \mathrm{e}^{i\omega_0 t} & 1 \end{array}\right)^t$. To 0th order in $k$ we find that in the first regime $\overline{m}_k = 2+\mathcal{O}\left(k^2\right)$, $\nu_{d\,k} = 2+\mathcal{O}\left(k^2\right)$; in the second regime $\overline{m}_k \simeq 0$ and $\nu_{d\,k} = 1+\mathcal{O}\left(k^2\right)$. The window in which the second regime holds (and in which $\nu_{d\,k}$ and $\overline{m}_k$ have a smaller value) tends to close up when $\omega_0$ approaches a zero $\omega_0^{[q]}$ of $J_0(2/\omega_0)$ in the same way as shown in Fig. 6. So, when $\omega_0 = \omega_0^{[q]}$ for some $q$, the first regime (in which $\nu_{d\,k}$ and $\overline{m}_k$ have a bigger value) holds even at the lowest values of $k$, therefore at these frequencies we have peaks in the integrals $\nu_d$ and $\overline{m}$.

## V. ISING CHAINS WITH LOCALIZED TRANSVERSE FIELD INHOMOGENEITY

In this section we consider in more detail the effect of breaking translational invariance as one would do, for instance, in trapped cold atomic systems. As we discuss in the main text, breaking translational invariance with a localized inhomogeneity leads at most to a finite number of discrete quasi-energies, while the vast majority of the spectrum is, in the thermodynamic limit, a continuous one. When this happens, the Riemann-Lebesgue lemma applies to the continuous part of the spectrum leading for long times to a periodic contribution which, in the thermodynamic limit, overwhelms the persisting fluctuations arising from the discrete quasi-energies. Nevertheless, not all operators reach a steady state, but just those which have a large number of non-vanishing matrix elements mostly among Floquet states in the continuous part of the spectrum.

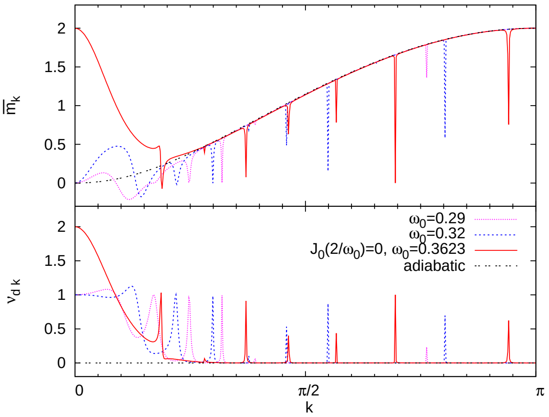


FIG. 8: The integrands $\overline{m}_k$ (upper panel) and $\nu_{d\,k}$ (lower panel) vs $k$ for the frequency $\omega_0^{[2]} \simeq 0.3623$ and some frequency nearby. Notice that the small $k$ behaviour of the integrand at the first frequency is very different from what happens at the other frequencies. For high $k$ the integrands are almost equal to their adiabatic value (reported for comparison) from which they differ just at the Floquet quasidegeneracies where they show narrow spikes.

To show this in detail, we apply the results of Section I to perform a calculation of an Ising system in which we superimpose to the transverse field considered so far a fixed-in-time but site-dependent Gaussian field

$$h_j(t) = 1 + h_G \mathrm{e}^{-(j-j_c)^2/2l^2} + A\cos(\omega_0 t) \tag{42}$$

with a certain (fixed) width $l$, and centered on the middle site $j_c = L/2+1$. The presence of such a site-dependent field creates discrete levels (and Floquet quasi-energies) below and above the standard spectral interval (see Fig. 9), where, however, the majority of the states accumulate in the thermodynamic limit to form a continuous spectrum. As it can be seen in the figure, this holds true at every frequency. In Fig. 3 of the main text we show that the space-average transverse magnetization (see Eqs. (8) and (9)) $m(t) = (1/L)\sum_j m_j(t)$ (upper right panel) sampled at the end of each period ($t = n\tau$) has fluctuations which decrease in magnitude as we make the chain longer: the fluctuations disappear in the thermodynamic limit. The transverse magnetization at the central site $j = L/2$ (lower right panel), in the middle of the inhomogeneity, shows fluctuations which do not decrease as we make the chain longer. We believe that this is due to the fact that this operator has matrix elements mostly among the Floquet-modes belonging to the

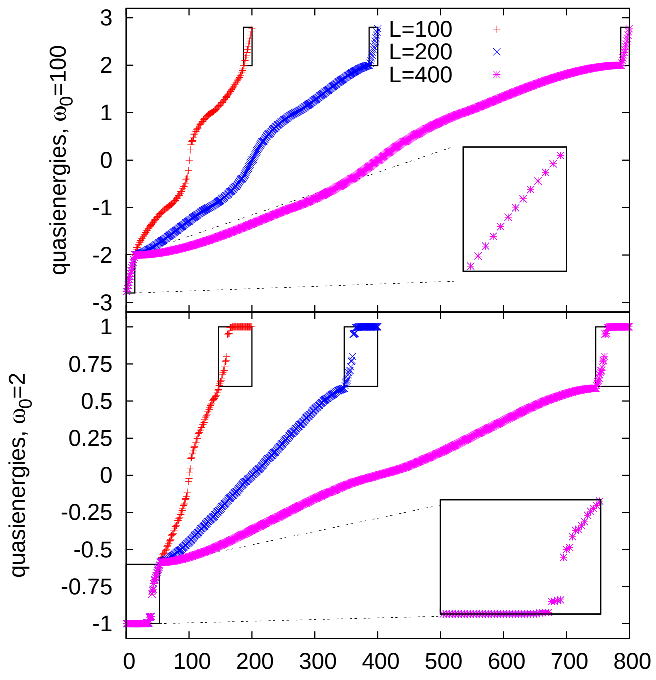


FIG. 9: The Floquet spectrum for $\sigma = 20$, $\widetilde{h} = 2.8$ (see Eq. (42)) $\omega_0 = 100$ (Upper panel) and $\omega_0 = 2$ (Lower panel). In both cases, above and below the continuous part of the spectrum, we notice the appearance of discrete quasienergies whose number does not change as the length of the chain increases (see inset). In abscissa, the progressive number of the quasienergies.

discrete part of the Floquet spectrum.

As a concluding remark, we show in Fig. 10 the Floquet spectrum at frequencies $\omega_0 = 100$ and $\omega_0 = 2$ for a $XX$ chain

$$\hat{H}(t) = -\frac{1}{2}\sum_{j=1}^{L}\left[\sigma_j^x\sigma_{j+1}^x + \sigma_j^y\sigma_{j+1}^y + h_j(t)\sigma_j^z\right] \ . \quad (43)$$

We remark the difference with Fig. 9: in the $XX$ case, when the frequency is lower than the width of the continuous part of the unperturbed energy spectrum, the discrete energy levels hybridize with the continuous ones thanks to resonant coupling; the resulting Floquet spectrum is strictly a continuum to which Riemann-Lebesgue lemma applies. This result is consistent with the findings of[11]. In that case, the Floquet spectrum was continuous for all frequencies because the unperturbed energy spectrum was unbounded from above. We do not understand why the Ising chain behaves so differently, this is a point which deserves further studies.

[1] T. Caneva, R. Fazio, and G. E. Santoro, Phys. Rev. B **76**, 144427 (2007).
[2] J. H. Shirley, Phys. Rev. **138**, B979 (1965).
[3] J. Hausinger and M. Grifoni, Phys. Rev. A **81**, 022117 (2010).
[4] M. Grifoni and P. Hänggi, Physics Reports **304**, 229 (1998).
[5] S. Bhattacharyya, A. Das, and S. Dasgupta, ArXiv e-prints (2011), 1112.6171.
[6] E. Lieb, T. Schultz, and D. Mattis, Annals of Physics **16**, 407 (1961).
[7] R. W. Cherng and L. S. Levitov, Phys. Rev. A **73**, 043614 (2006).
[8] A. Das, Phys. Rev. B **82**, 172402 (2010).
[9] A. Russomanno, S. Pugnetti, V. Brosco, and R. Fazio, Phys. Rev. B **83**, 214508 (2011).
[10] Y. Kayanuma, Phys. Rev. A **50**, 843 (1994).
[11] K. Yajima, Commun. Mat. Phys. **87**, 331 (1982).
[12] We notice that it would be easy to implement the coherent evolution of a system initially in thermal equilibrium at temperature $T = 1/(k_B\beta)$, by imposing at time 0 $\left\langle\gamma_{d\,\alpha}(0)^\dagger\gamma_{d\,\alpha}(0)\right\rangle_0 = \frac{1}{1+e^{-\beta E_\alpha(0)}}$ and going on with the following analysis.

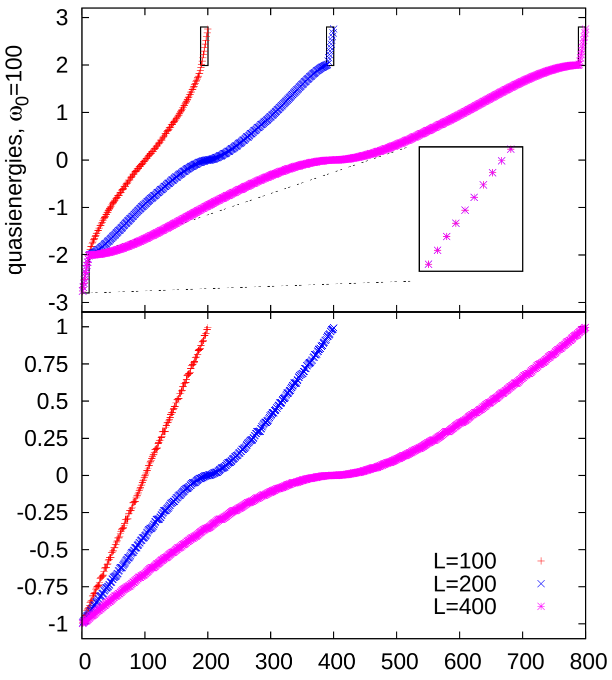


FIG. 10: The Floquet spectrum for the $XX$ chain (see Eq (43)) $\sigma = 20$, $\widetilde{h} = 2.8$ (see Eq. (42)) $\omega_0 = 100$ (Upper panel) and $\omega_0 = 2$ (Lower panel). In the upper panel, above and below the continuous part of the spectrum, we notice the appearance of discrete quasienergies whose number does not change as the length of the chain increases (see inset). This does not happen at $\omega_0 = 2$ in the lower panel, it is smaller than the width of the continuous part of the spectrum. In abscissa, the progressive number of the quasienergies.
